# Supplementary material for: Distributed Decisions on Optimal Load Balancing in Loss Networks
Source: arXiv:2307.04506 source file (2023-07-17)
Supplement: Supplementary file 1 [file appendix.tex]

\appendix
\section{Supplementary Material}
\subsection{Proof of Theorem \ref{thm:cha}}
\label{appenddix_theorem3_1}
Given an arbitrary strategy profile $\mathbf p$, define $(V_1,V_2,V_3,V_4)$ as a partition of $N$, where $V_1=\{i\in N_1~|~p_i=1\}$,  $V_2=\{i\in N_1~|~p_i=0\}$, $V_3=\{j\in N_2~|~p_j=1\}$ and $V_4=\{j\in N_2~|~p_j=0\}$. Clearly, all users in $V_1$ and $V_3$ choose DP, and all users in $V_2$ and $V_4$ choose IP.  Supposing $\mathbf p$ is a NE, we discuss the deviation of users in $V_1,V_2,V_3,V_4$ respectively. 
\begin{proof}
Given $\mathbf p$, let $(V_1,V_2,V_3,V_4)$ be a partition of $N$ as defined above. We discuss the four cases. 

\textbf{Case 1.} When (a) $u_1=n_1$ and $u_2<n_2$,  $V_4$ is nonempty. If $\mathbf p$ is a NE, it must satisfy Eq. (\ref{eq:c4}), that is, $2\bar{q}u_2\ge q\mu/\phi+n_1(1+\bar{q}^2)+(n_2-1)\bar{q}-n_1\bar{q}^2=q\mu/\phi+n_1+(n_2-1)\bar{q}$. However, because $\bar{q}u_2\le n_1,\bar{q}u_2\le (n_2-1)\bar{q}$ and $q\mu/\phi>0$, it cannot hold. 

When (b) $u_1=0$ and $u_2>0$, $V_2$ is nonempty. If $\mathbf p$ is a NE, it must satisfy Eq. (\ref{eq:c2}), that is, $u_1\ge t_1(u_1)-1$. It follows that $0=2\bar{q}u_1\ge q\mu/\phi+u_2(1+\bar{q}^2)+(n_1-1)\bar{q}-n_2\bar{q}^2\ge q\mu/\phi+1+(n_1-1)\bar{q}-(n_2-1)\bar{q}^2\ge q\mu/\phi+1>0$, a contradiction. 

\smallskip\textbf{Case 2.} When $u_1\in[0,n_1),u_2\in[0,n_2)$, $V_2$ and $V_4$ are nonempty.  $\mathbf p$ is NE if and only if  (\ref{eq:c2}) and (\ref{eq:c4}) are satisfied simultaneously. Noted that Eqs.~(\ref{eq:c1}) and (\ref{eq:c3}) do not matter in Case 2, because (\ref{eq:c2}) and (\ref{eq:c4}) are satisfied when $\mathbf p$ is NE.

\smallskip\textbf{Case 3.} When $u_2=n_2,u_1\in(0,n_1)$, $V_1,V_2,V_3$ are nonempty, and $V_4$ is empty.  $\mathbf p$ is NE if and only if (\ref{eq:c1}) (\ref{eq:c2}) and (\ref{eq:c3}) are satisfied simultaneously. The sufficiently and necessary condition only needs (\ref{eq:c1}) and (\ref{eq:c2}), that is, $u_1\in[t_1(u_2)-1,t_1(u_2)]$.

\smallskip\textbf{Case 4.} When $u_1=n_1,u_2=n_2$, $V_1,V_3$ are nonempty, and $V_2,V_4$ are empty.  $\mathbf p$ is NE if and only if (\ref{eq:c1}) and (\ref{eq:c3}) are satisfied, that is, $2\bar{q}n_1\le q\mu/\phi+n_2(1+\bar{q}^2)+(n_1+1)\bar{q}-n_2\bar{q}^2$ and $2\bar{q}n_2\le q\mu/\phi+n_1(1+\bar{q}^2)+(n_2+1)\bar{q}-n_1\bar{q}^2$. It is easy to see that, (\ref{eq:c1}) and (\ref{eq:c3}) are equivalent to $n_1\bar{q}\le q\mu/\phi+n_2+\bar{q}$.

\smallskip Note that every situation of $u_1,u_2$ is included in the above four cases. So we complete a characterization.
\end{proof}
